# Supplementary material for: Unstable drainage dynamics during multiphase flow across capillary heterogeneities
Source: arXiv:2511.04862 source file (2025-11-06)
Supplement: Supplementary file 1 [file SI_ArXiv.pdf]

# Supporting information document for 'Unstable drainage dynamics during multiphase flow across capillary heterogeneities'

Catrin Harris[a], Samuel Krevor[a], Ann H. Muggeridge[a], Michael Camilleri[b], Samuel J. Jackson[b*]

[a] Department of Earth Science and Engineering, Imperial College London, London, UK.
[b] CSIRO Energy, Clayton North, Victoria, Australia.

## Abstract

This document serves as detailed supporting information for the main paper, providing extra analysis and figures to support the main findings. We note that figures, equations, tables and associated references from the supporting information contain the prefix S. All references without the S prefix refer to the main document.

## S1 Experimental Methodology

The experimental setup is detailed in Figure S1. Three ISCO Teledyne pumps are used to inject fluid (injection pump), maintain pressure (back pressure pump) and confine the core (confining pump). The pore pressure is maintained from the outlet through the back pressure pump and a high-pressure regulator. The experiment was carried out with the experimental pore pressure maintained at 4 MPa and an overburden pressure 7 MPa confining the core. The temperature was 22.5 ± 0.6 °C and 22.3 ± 0.1 °C for the ANSTO R1 and ANSTO R2 experiments respectively. A 500ml equilibration vessel is used to pre-equilibrate the $N_2$ and brine at experimental conditions (4 MPa, room temperature) prior to injection for ∼ 12 hours.

An outline of the experimental methodology followed in this experiment is provided below. A similar experimental setup and methodology are described in [1], [2], [3].

1. The core sample is placed into a viton sleeve, with core sized to fit using a layer of shrink wrap. The core is secured by 2 end-caps and loaded into the PEEK core-holder (custom designed, $\phi$12.5 mm RS Systems).
2. A net overburden pressure of 3 MPa is applied to prevent fluid bypass of the core.
3. After configuring the beamline setup to achieve suitable resolution and contrast, a dry scan of the core is taken.
4. The core is fully saturated with brine (∼ 20 pore volumes injected). The pore pressure is increased to 4 MPa using the back pressure pump, with the confining pressure increased to 7 MPa to keep a constant net overburden pressure. A scan of the brine saturated core is taken.

*Corresponding author: Samuel J. Jackson, samuel.jackson@csiro.au

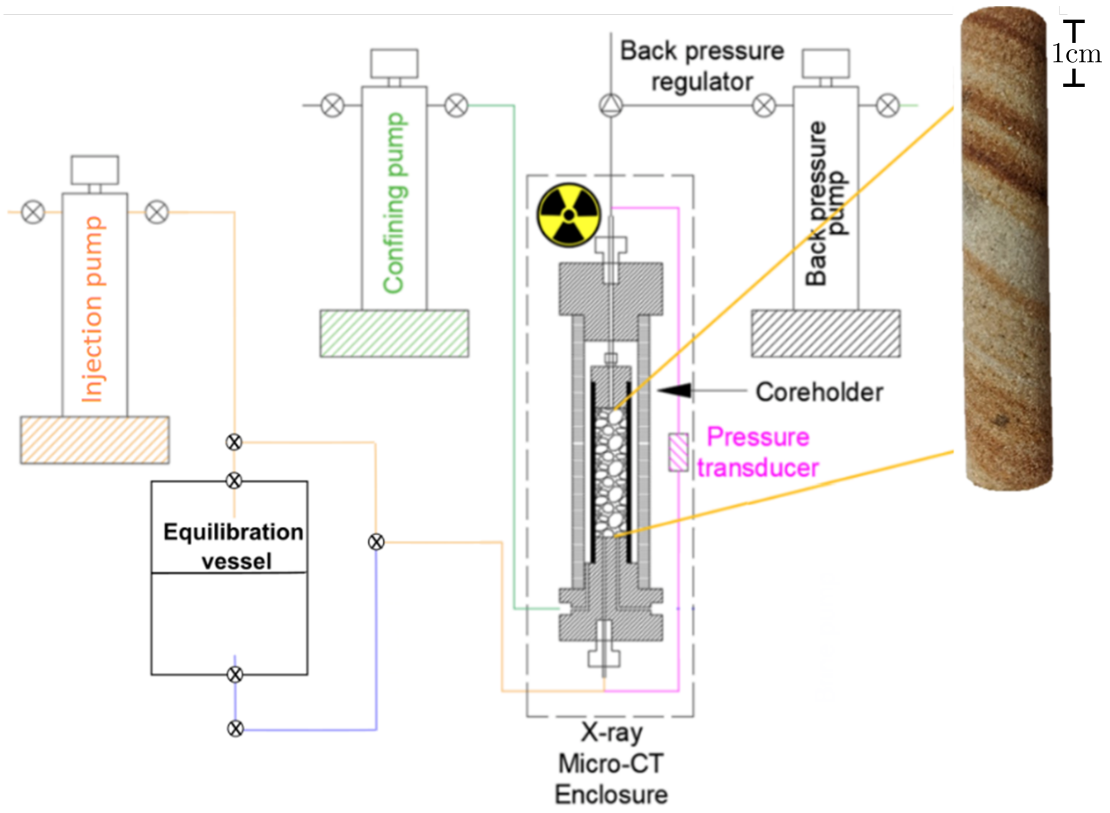


Figure S1: Schematic of the experimental setup used at ANSTO.

5. Due to the low flow rates, and relatively large dead volume in the setup, the injected fluids are first flushed through the bypass line at approximately 10 ml/min. This ensures the inlet line is filled with the appropriate injection phase. The flow rate is then reduced to match the injection rate, and time elapsed to allow the pressure to equilibrate with the intended pore-pressure of the sample.

6. Nitrogen is injected into the core at a rate outlined in Table S1. The differential pressure response (Keller, 0.35 bar) was used to determine when the injected phase had reached the core inlet. From this time, continuous full core scans are taken to track $N_2$ distribution through the core until post breakthrough. The fluids are injected as per the timings detailed in Table S1, based on pressure response and practical time constraints.

7. The core is flushed with $CO_2$, directly from the gas cylinder, until dry, verified through scans.

8. Brine is then flushed through the bypass and core to dissolve the $CO_2$ and re-saturate the core with brine. A scan is taken of the fully saturated brine system to confirm the core has been properly flushed.

9. Steps 5–8 are repeated over the flow rates detailed in Table S1.

The pore volume injected, PVI, is calculated as a dimensionless volume,

$$\mathrm{PVI} = \frac{V}{V_p} = \frac{t \cdot q}{V_p} \tag{S1}$$

where $V$ is the total fluid volume injected and $V_p$ is the pore volume of the rock. The time injected $t$ is the difference in time between the scan midpoint and the start of injection defined by the characteristic

pressure spike, and $q$ is the injection rate. Negative values of PVI are reported for scans taken before the injected fluid reached the core inlet.

| Experiment name | Rate [ml/min] | Capillary number | Repeat name | Injection duration | | |
|---|---|---|---|---|---|---|
| | | | | [min] | [PVI] | [# scans] |
| HF | 0.1 | $4.9 \text{x} 10^{-9}$ | R1 | 60 | 3.82 | 8 |
| | | | R2 | 140 | 8.86 | 18 |
| LF | 0.01 | $4.9 \text{x} 10^{-10}$ | R1 | 180 | 1.33 | 28 |
| | | | R2 | 240 | 1.64 | 32 |

Table S1: Experiments performed with associated flow rate and pore-scale capillary number [4]. The duration of fluid injection is displayed in minutes and pore volumes injected (PVI), with the number of scans taken listed.

At the experimental conditions, the brine and $N_2$ are estimated to have viscosity's of $\mu_w = 7.83 \text{x} 10^{-4}$ Pa·S [5], [6] and $\mu_{N_2} = 1.83 \text{x} 10^{-5}$ Pa·S [7], and densities of 1023 kg/m$^3$ [8] and 45.8 kg/m$^3$ [7], respectively. The fluids have an interfacial tension of $\gamma = 69.8$ mN/m for the pure DI water-$N_2$ system [9], with maximum ± 0.5 mN/m for the addition of small KI salt concentrations to the water [10].

The pore-scale capillary number,

$$N_c = \frac{q\mu}{\gamma}, \tag{S2}$$

with $q$ Darcy velocity, $\mu$ viscosity of invading phase, $\gamma$ interfacial tension, for each experiment is detailed in Table S1, is key to understanding the controlling force influencing the flow dynamics. At the pore-scale, capillary numbers less than $10^{-4}$ are indicative of capillary dominated fluid distributions within the pores [5]. The fraction of intermittent flow pathways is dependent on the capillary number and viscosity ratio [11]. The viscosity ratio is defined as the ratio of the viscosity of the non-wetting phase to the wetting phase; $M = \mu_{nw}/\mu_w \sim 0.023$ [11], [12]. The experimental values meet the critical threshold for intermittent fluid connectivity, and as such dynamic connectivity is expected [4].

## S1.1 Verification of Volume Flux

The effective flow rate is calculated for the low flow rate experiments during breakthrough, Table S2. The effective flow rate is calculated from the volume of $N_2$ in the segmented images and injection period, averaged over the number of scans available. In order to minimise error, scans where stitching clearly impacts (i.e. scan time is comparable to fluid movement) are removed from the average.

| Experiment | Effective Rate [ml/min] | Std Dev [ml/min] | Number of scans used | Rate [ml/min] | Relative difference |
|---|---|---|---|---|---|
| R1 LF | 0.009 | 0.002 | 9 | 0.01 | 10% |
| R2 LF | 0.008 | 0.004 | 19 | 0.01 | 20% |

Table S2: The average effective flow rate for each experiment calculated from number of scans listed. The effective flow rate is compared with the pump flow rate injected into the sample. The standard deviation and range in the calculated effective flow rate across the scans used are given.

These results show that the flow rate is constant macroscopically, within the error from calculating the volumetric flux. Therefore the inlet condition may be considered identical from a continuum perspective

(constant flow). The two-phase flow is very sensitive to perturbations in the boundary conditions, therefore small differences in experimental conditions may lead to discrepancies in the observed fluid distributions.

### S1.2 Scanning Setup

The synchrotron radiation in-situ computed tomography performed at the Australian synchrotron used the Imaging and Medical beamline (IMBL). Hutch 3B was used, with source to sample length of $\sim$ 135 m. The setup used a monochromatic beam at 60 keV. A ruby detector at 20 micron resolution was used to image around 4000 projections, each with 0.03 s exposure time. The total rock volume was imaged in three vertical sections, stitched together.

Two repeated trapping experiments were carried out at ANSTO with similar IMBL beamline setup. Repeat 1 used a magnetic flux of 4 T, whilst repeat 2 used a lower magnetic flux of 3 T, as one of the superconducting magnets quenched so the full magnetic flux could not be used. The same imaging protocol was used, with some of the beam filters removed, resulting in a photon flux reduced by approximately 20%, increasing the noise by approximately 4.5% ($signal\ to\ noise\ ratio = \sqrt{number\ of\ detected\ photons}$) [13].

Using the setup outlined, we achieved time resolution of 7 minutes to scan the full core ($\sim$ 6 cm), with resolution of $\sim$ 20μm (Day 1: 20.4 μm, Day 2: 19.1 μm $\pm$ 0.2 μm). An automatic image reconstruction pipeline was developed at ANSTO to stitch the images, denoise, and remove ring artefacts from the images. After postprocessing and converting to 8 bit, each image was approximately 2 Gb in size. Around 100 time-resolved image cycles were captured for each repeat experiment, generating around 0.4 Tb of data in total.

## S2 Image Processing Workflow

At Imperial College London, the data was processed on an Intel Xeon Gold 5118 CPU, utilising a machine with 256 Gb RAM. The processing was carried out in Avizo v2019 and v2023. Firstly, a time series of the full core registered in space was created. A major challenge of time-lapse CT is ensuring the exact alignment of images taken at different time intervals [14]. The ANSTO data constituted a time series containing raw greyscale images of the full core, each $\sim$ 2 Gb. Images were registered in space, relative to a high-resolution dry scan, and re-sampled with an equivalent voxel size, 20 μm between repeats.

To create binarised images of the different phases, the images were subjected to a non-local means edge preserving filter to reduce image noise (increase signal to noise ratio [15]), before a segmentation algorithm was applied. An extensive testing of the post processing workflow was carried out to identify the most appropriate segmentation method and settings for the sample. To achieve the high levels of automation required to process images of this size and number, Tcl scripts were developed to automate the Avizo processing workflow.

To accurately quantify the porosity, the ANSTO dry scan (4000 projections) taken prior to the in-situ flow experiment was used. Porosity segmentation is more direct than multiphase flow segmentation due to the higher contrast and signal to noise ratio. To extract the porosity from the dry scan, the image was subjected to a non-local means filter. A watershed segmentation was then used to segment the pore space [5]. To segment the dry image; first a gradient image of the dry scan is produced. This is used along with the input image to produce a correlation histogram from which appropriate seeds are assigned. These seeds are used in Avizo's marker-based watershed algorithm, with the segmentation labels expanded to fill the catchment basins, until the entire pore space is segmented. The porosity has not been over segmented to match external measures, and therefore is lower than calculated through medical CT due to the sub-resolution porosity not captured [5], [16].

The following section outlines segmentation methods applied during the post processing of multiphase images. A lower contrast is observed in the fluid scan, compared with the dry scan, due to brine in the system resulting in increased X-ray attenuation. Simple thresholding of the images was also performed and found to produce more noisy and less physical results, due to the shape of the pores not being accounted for during the segmentation algorithm.

Although most segmentation algorithms are biased based on subjective user inputs, Leu et al.'s (2014) sensitivity study showed watershed algorithms were the most robust [17], [18]. In addition, a watershed algorithm can reduce partial volume effects, which result from the greyscale value of a reconstructed voxel being averaged over its volume [5], [15], [19]. As such, a watershed segmentation workflow was used to segment the multi-phase filtered image, applying a similar workflow to the porosity segmentation.

Firstly the image gradient was calculated. The optimal seeds to segment the $N_2$ were defined from the correlation histogram, as to assign enough of the pore space that catchment basins would correctly fill on segmentation whilst minimising any falsely assigned seeds. Segmenting the non-wetting phase is less sensitive to image processing than the wetting phase, as the $N_2$ has a more distinct greyscale value to the grain and typically occurs in the centre of large pores [17]. The image was then subject to Avizo's watershed segmentation algorithm, with labels expanded until the whole image was assigned.

A noise removal was performed, to produce the final segmented $N_2$ phase. In order to estimate a maximum size for noise removal, the Young-Laplace equation was used to calculate the smallest pore radius that a terminal meniscus of $N_2$ can invade, based on the maximum capillary pressure of the system. The maximum capillary pressure for Bentheimer is estimated as 4.5 kPa from Jackson and Krevor 2020 (Supporting Information, Figure 7) based on final non-wetting phase saturations [3]. Assuming perfect non-wetting and an interfacial tension $\gamma$ between fluid phases of $6.98 \text{x} 10^{-2}$ N/m, the minimum radius of invasion is, $r = \frac{2\gamma}{P_c} = 31 \mu m$. Based on the scan resolution, this is equivalent to 1.6 voxels in the ANSTO data, corresponding to a volume of $\sim 4$ voxels$^3$. $N_2$ spots less than this size, below the minimum pore size invaded, were removed post-segmentation to denoise the image.

The $N_2$ segmented images were masked with the pore space, calculated from the dry scan. The core is fully saturated, hence brine is defined as the remaining phase after $N_2$ segmentation is completed.

## S2.1 Segmentation Challenges

Various artefacts in the images, alongside noise inherent to the scans, add complexity to the image segmentation. These include ring artefacts likely generated through defects in the detector array and streak artefacts caused by highly attenuating inclusions, which may cause segmentation artefacts [13], [19]. To obtain high quality images, the internal processes should be much slower than the scanning time. Fluid movement faster than the timescale of observation manifests as image artifacts in the reconstructed image [20]. However, there is a trade-off between acquisition time and image quality, as to obtain a good signal-to-noise ratio an appropriate exposure time is necessary [19]. Fluid movement during the scan, resulting from the relatively long scan time compared to the flow rate, introduces error into the segmentation. A high-quality image is taken to evaluate the detailed structure of the sample, before acquiring fast images to capture the dynamic processes.

The nitrogen dynamics during drainage are largely controlled by the rate of injection. During drainage at high flow rate, $N_2$ reaches the core outlet before the first scan completes. The nonphysical distribution of the $N_2$ saturation in the first scan results from the movement of $N_2$ during the scan time, when the drainage front advances through the core over a similar time interval to that taken to scan the full core. In contrast, during drainage at low flow rate, the evolution of the saturation is captured over multiple

scans before nitrogen reaches the core outlet.

The greatest fluid movement is observed during breakthrough of the $N_2$ phase. A change in pore occupancy during the scan results in intermediate grey-scale values, between the brine and $N_2$ grey-scale peaks [21]. The grey-scale value is dependent on the time during the scan that the pore is occupied by each phase. As the imaging protocol was not optimised to segment intermediate grey-scale values, the fluid was segmented as $N_2$ if within the segmentation threshold or otherwise considered as brine. Future studies imaging dynamic processes at a relatively long scan time should consider optimising brine/$N_2$ contrast, to allow for segmentation of intermittent phases.

# S3 Saturation Built Up at the Heterogeneity

## S3.1 3D Saturation Distribution

The underlying topology of the pore space influences core-scale saturation distributions. The $N_2$ saturation distribution at the end of drainage is displayed as a 3D volume rendering, with the brine and rock phases excluded. The impact of heterogeneity is demonstrated in the 3D volume rendering of the $N_2$ saturation distribution for the R1 experiment at the end of high and low flow rate drainage (Figure S2a,b). The flow of $N_2$ through the core is controlled in both cases by just a few pores within the heterogeneous layer of the rock, channelling flow through the main heterogeneity (two-thirds of the way along the core length). The fluid distribution varies with flow rate, highlighting the impact of the capillary number on the role of heterogeneity within a system.

A few pores control flow through the dominant heterogeneity both during the R2 high and low flow rate experiments, as shown in the 3D volume rendering of the $N_2$ saturation distribution at the end of drainage (Figure S2c,d). More pores within the heterogeneity are $N_2$ saturated in the R2 than in the R1 experiment, however, this additional filling of the pores only occurs at late times when high numbers of pore volumes of $N_2$ have been injected.

## S3.2 Pore-scale Capillary Barrier

The magnitude of the capillary pressure barrier resulting from the heterogeneity, depends on a small subset of throats which control breakthrough of the heterogeneity barrier. The pores which fill in the scan prior to breakthrough are identified and compared to those filled post breakthrough. The resulting difference images are shown in Figure S3. This allows the connecting throats to be analysed at the scale of individual pores, with the throat adjacent to the most downstream pore filled prior to breakthrough identified. In the low flow rate R2 experiment, $N_2$ breaches the capillary pressure barrier through a different region of the pore space. Qualitatively, the upstream region of the pore space fills beyond the barrier identified in the R1 experiment, with more pore volumes of $N_2$ injected, the $N_2$ finds a different path across the low porosity layer (Figure S3).

In Figure S4, the pore-space controlling breakthrough of the heterogeneity barrier in the R1 low flow rate experiment is shown at the pore-scale (large pore at centre of images demonstrates the connection of interest). Prior to breakthrough the left-hand side of the pore is observed to fill with $N_2$ but is prevented from fully filling by the capillary entry pressure of the adjacent downstream throat.

The absence of blur and intermediate grey within the images highlights the steady saturation, and limited intermittency, over the scanning interval (7 minutes), demonstrating the build-up in $N_2$ at the throat clearly. Figure S5 is used to measure the diameter of the controlling throat.

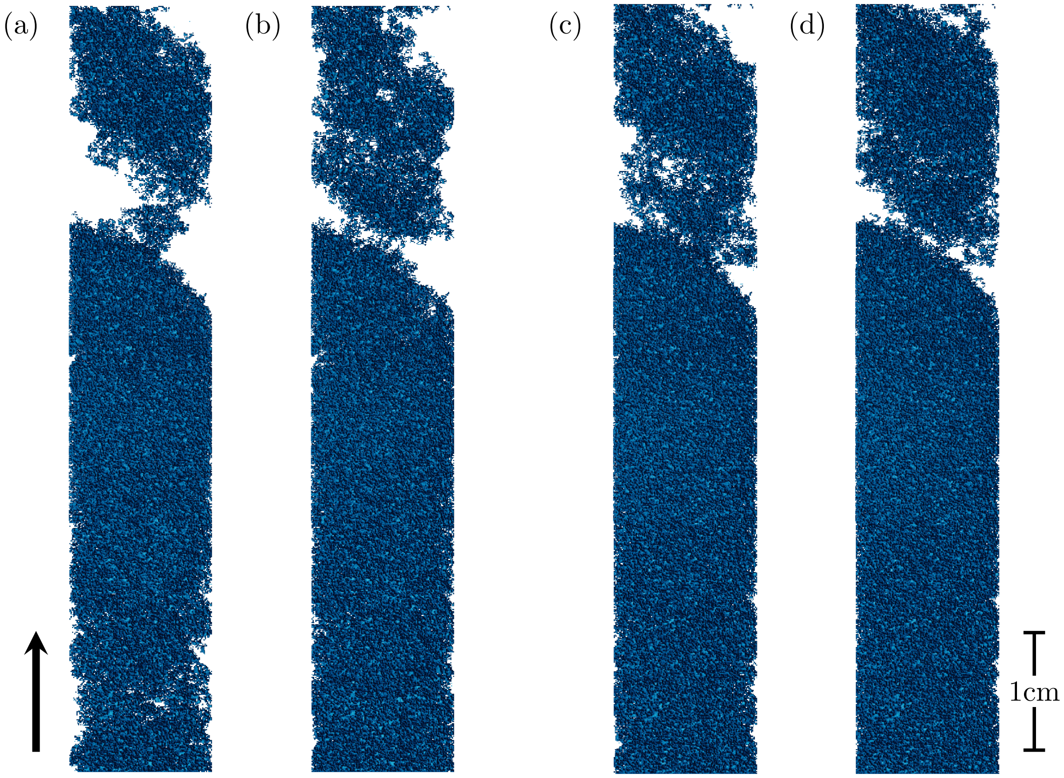


Figure S2: 3D volume rendering of $N_2$ saturation distribution of R1 at the end of drainage (a) high flow rate (3.82 pore volumes), (b) low flow rate (1.33 pore volumes), and R2 at the end of drainage (c) high flow rate (8.86 pore volumes), (d) low flow rate (1.64 pore volumes) (XZ view).

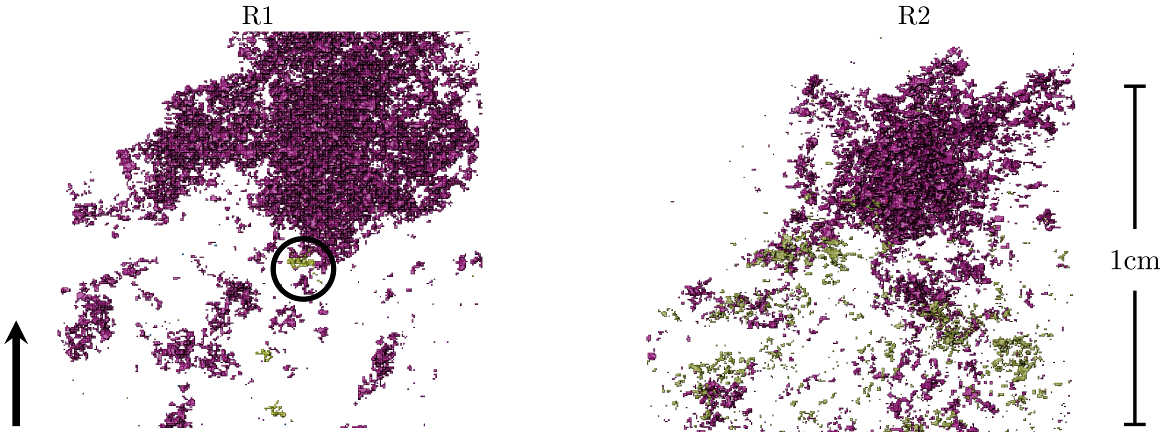


Figure S3: Low porosity region within the low flow rate experiment showing 3D volume rendering of the difference saturation between scans during heterogeneity breakthrough. The yellow volume shows the difference in saturation in the scan prior to breakthrough ($t_{prior}$-$t_{prior\text{-}1}$) and the pink volume the difference in saturation during the breakthrough scan ($t_{breakthrough}$-$t_{prior}$). The connection of interest is marked in the R1 experiment.

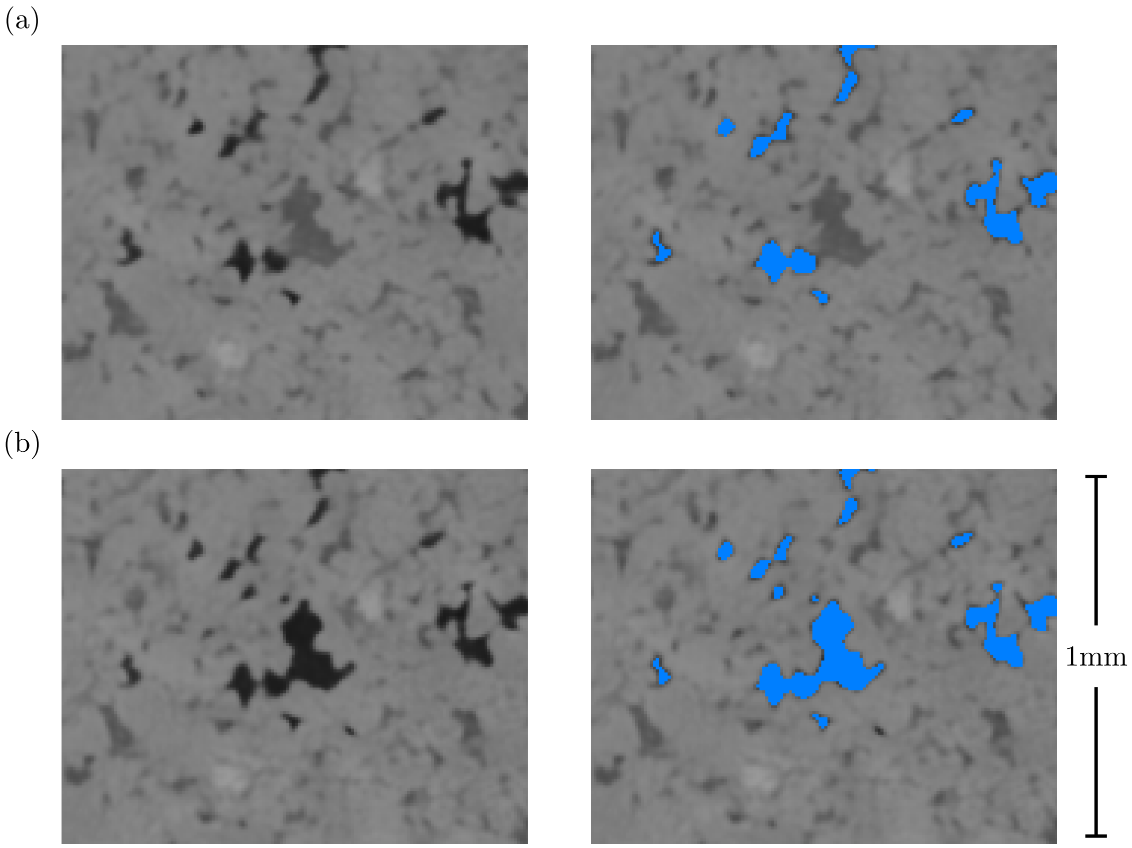


Figure S4: Connecting throat (image centre) in heterogeneity region during R1 low flow rate drainage experiment, showing the greyscale image and overlaid $N_2$ segmentation, (a) before (0.41 pore volumes injected) and (b) after (0.46 pore volumes injected) the heterogeneity is breached.

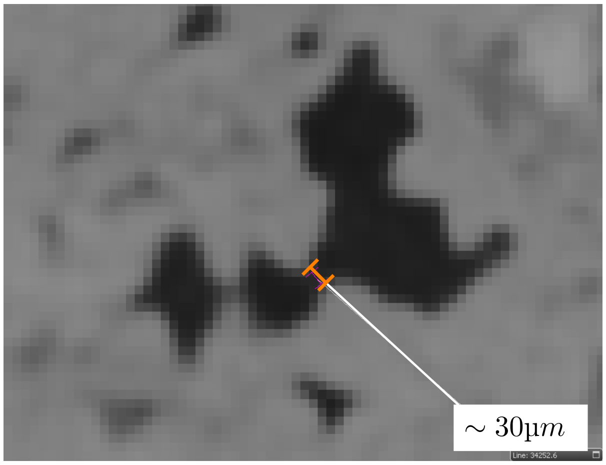


Figure S5: Connecting throat in heterogeneity region during R1 low flow rate experiment, with diameter measurement overlaid.

### S3.3 Magnitude of Continuum-scale Saturation

Whilst the distribution of the saturation is determined by the ratio of capillary to viscous forces, the magnitude of the saturation built up at the heterogeneity is determined by the difference in capillary entry pressure between the layers [22], [23]. Together, these parameters establish the total saturation trapped. Table S3 outlines the critical saturation build-up at the major heterogeneity perpendicular to flow. The heterogeneity occurs as a gradation in grain size at the transition zone, with a gradual build up of $N_2$ observed, dependant on the heterogeneity distribution. The critical saturation therefore does not occur as a sharp interface but instead develops over the distance given in Table S3. This highlights the complexity in modelling real rock samples, where sharp interface conditions do not apply at the pore-scale.

| Experiment | Rate [ml/min] | Max $N_2$ saturation | $\Delta N_2$ saturation built up | Distance [cm] | Saturation gradient [cm$^{-1}$] |
|---|---|---|---|---|---|
| ANSTO R1 | 0.1 | 0.58 | 0.57 | 1.74 | 0.33 |
| | 0.01 | 0.58 | 0.48 | 1.61 | 0.30 |
| ANSTO R2 | 0.1 | 0.62 | 0.51 | 1.61 | 0.32 |
| | 0.01 | 0.65 | 0.53 | 1.61 | 0.33 |

Table S3: Critical slice average $N_2$ saturation build up at a heterogeneity at the end of drainage. The saturation gradient between the high and low capillary pressure zones is detailed, showing deviations from a sharp interface.

The $\Delta N_2$ saturation built up is calculated from the maximum saturation relative to the baseline saturation at the heterogeneity. The distance over which the build-up occurs is dependant on the heterogeneity within the sample. It is observed that the maximum saturation and associated net saturation build-up is similar within each experiment performed on the sample. The critical saturation build-up results from the difference in capillary entry pressure across the heterogeneity. As this depends on the geology of the sample itself, it is expected that the critical saturation should be similar across the same sample with different flow conditions. Small differences in critical saturation result from experimental uncertainty and variations in flow path.

## S4 Differential Pressure

The differential pressure over the core was measured for the different experiments, displayed in Figure S6. The data is corrected for shift in the Y-axes relative to a zero baseline. The X-axes is displayed as a time interval relative to the point fluid reached the core inlet, identified by the characteristic pressure spike. The scan timestamp is overlaid, with the start time of the scans shown as dashed vertical lines.

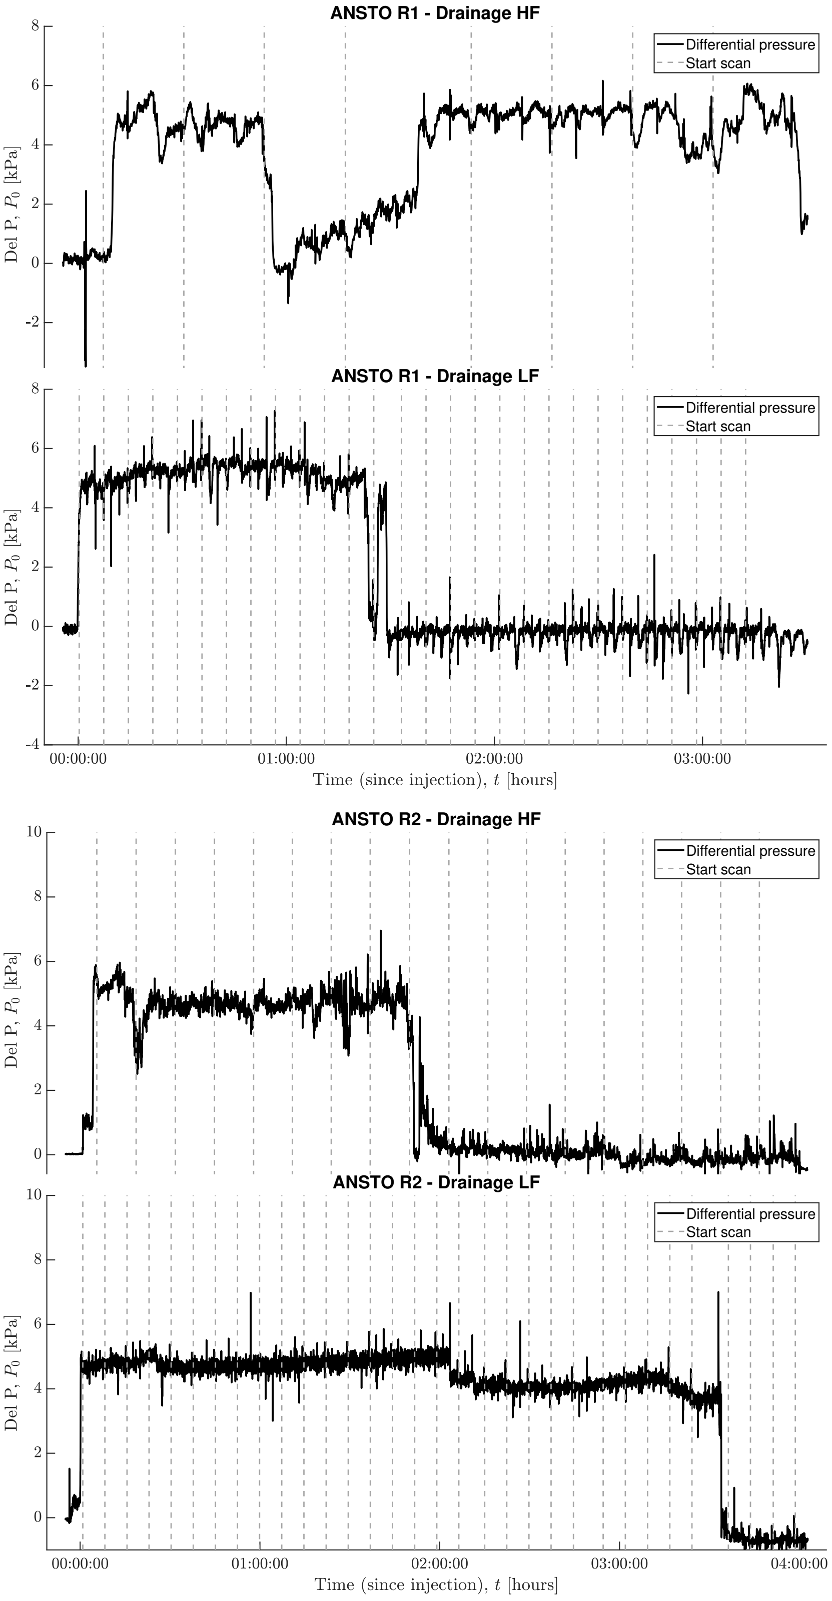


Figure S6: Differential pressure over LF and HF R1 & R2 experiments, with start of scan timestamp marked.

# References


[1] C. A. Reynolds and S. Krevor, "Characterizing flow behavior for gas injection: Relative permeability of $CO_2$-brine and $N_2$-water in heterogeneous rocks," *Water Resources Research*, vol. 51, no. 12, pp. 9464–9489, 2015. DOI: 10.1002/2015WR018046.

[2] S. J. Jackson, S. Agada, C. A. Reynolds, and S. Krevor, "Characterizing Drainage Multiphase Flow in Heterogeneous Sandstones," *Water Resources Research*, vol. 54, no. 4, pp. 3139–3161, 2018. DOI: 10.1029/2017WR022282.

[3] S. J. Jackson and S. Krevor, "Small-Scale Capillary Heterogeneity Linked to Rapid Plume Migration During CO2 Storage," *Geophysical Research Letters*, vol. 47, no. 18, e2020GL088616, 2020. DOI: 10.1029/2020GL088616.

[4] C. A. Reynolds, H. Menke, M. Andrew, M. J. Blunt, and S. Krevor, "Dynamic fluid connectivity during steady-state multiphase flow in a sandstone," *Proceedings of the National Academy of Sciences*, vol. 114, no. 31, pp. 8187–8192, 2017. DOI: 10.1073/pnas.1702834114.

[5] S. J. Jackson, Q. Lin, and S. Krevor, "Representative Elementary Volumes, Hysteresis and Heterogeneity in Multiphase Flow From the Pore to Continuum Scale," *Water Resources Research*, vol. 56, no. 6, e2019WR026396, 2020. DOI: 10.1029/2019wr026396.

[6] D. E. Goldsack and R. C. Franchetto, "The viscosity of concentrated electrolyte solutions. II. Temperature dependence," *Canadian Journal of Chemistry*, vol. 56, no. 10, pp. 1442–1450, 1978, ISSN: 0008-4042. DOI: 10.1139/v78-236.

[7] R. Span, E. W. Lemmon, R. T. Jacobsen, W. Wagner, and A. Yokozeki, "A Reference Equation of State for the Thermodynamic Properties of Nitrogen for Temperatures from 63.151 to 1000 K and Pressures to 2200 MPa," *Journal of Physical and Chemical Reference Data*, vol. 29, no. 6, pp. 1361–1433, 2000. DOI: 10.1063/1.1349047.

[8] S. Al Ghafri, G. C. Maitland, and J. P. M. Trusler, "Densities of Aqueous $MgCl_2$(aq), $CaCl_2$(aq), KI(aq), NaCl(aq), KCl(aq), $AlCl_3$(aq), and (0.964 NaCl + 0.136 KCl)(aq) at Temperatures Between (283 and 472) K, Pressures up to 68.5 MPa, and Molalities up to 6 $mol \cdot kg^{-1}$," *Journal of Chemical and Engineering Data*, vol. 57, no. 4, pp. 1288–1304, 2012. DOI: 10.1021/je2013704.

[9] W. Yan, G. Y. Zhao, G. J. Chen, and T. M. Guo, "Interfacial Tension of (Methane + Nitrogen) + Water and (Carbon Dioxide + Nitrogen) + Water Systems," *Journal of Chemical and Engineering Data*, vol. 46, no. 6, pp. 1544–1548, 2001. DOI: 10.1021/je0101505.

[10] R. Aveyard and S. M. Saleem, "Interfacial tensions at alkane-aqueous electrolyte interfaces," *Journal of the Chemical Society, Faraday Transactions 1: Physical Chemistry in Condensed Phases*, vol. 72, no. 9, pp. 1609–1617, 1976. DOI: 10.1039/F19767201609.

[11] C. Spurin, T. Bultreys, B. Bijeljic, M. J. Blunt, and S. Krevor, "Mechanisms controlling fluid breakup and reconnection during two-phase flow in porous media," *Physical Review E*, vol. 100, no. 4, p. 043 115, 2019. DOI: https://doi.org/10.1103/PhysRevE.100.043115.

[12] C. A. Reynolds, "Two-phase flow behaviour and relative permeability between $CO_2$ and brine in sandstones at the pore and core scales," Ph.D. dissertation, Imperial College London, 2016.

[13] F. R. Verdun et al., "Image quality in CT: From physical measurements to model observers," *Physica Medica*, vol. 31, no. 8, pp. 823–843, 2015. DOI: 10.1016/j.ejmp.2015.08.007.

[14] T. Bultreys, W. De Boever, and V. Cnudde, "Imaging and image-based fluid transport modeling at the pore scale in geological materials: A practical introduction to the current state-of-the-art," *Earth-Science Reviews*, vol. 155, pp. 93–128, 2016. DOI: 10.1016/j.earscirev.2016.02.001.

[15] H. P. Menke, "Reservoir condition pore-scale imaging of reaction," Ph.D. dissertation, Imperial College London, 2016.

[16] Q. Lin, Y. Al-Khulaifi, M. J. Blunt, and B. Bijeljic, "Quantification of sub-resolution porosity in carbonate rocks by applying high-salinity contrast brine using X-ray microtomography differential imaging," *Advances in Water Resources*, vol. 96, pp. 306–322, 2016. DOI: 10.1016/j.advwatres.2016.08.002.

[17] G. Garfi, C. M. John, S. Berg, and S. Krevor, "The Sensitivity of Estimates of Multiphase Fluid and Solid Properties of Porous Rocks to Image Processing," *Transport in Porous Media*, vol. 131, no. 3, pp. 985–1005, 2020. DOI: 10.1007/s11242-019-01374-z.

[18] L. Leu, S. Berg, F. Enzmann, R. T. Armstrong, and M. Kersten, "Fast X-ray Micro-Tomography of Multiphase Flow in Berea Sandstone: A Sensitivity Study on Image Processing," *Transport in Porous Media*, vol. 105, no. 2, pp. 451–469, 2014. DOI: 10.1007/s11242-014-0378-4.

[19] V. Cnudde and M. N. Boone, "High-resolution X-ray computed tomography in geosciences: A review of the current technology and applications," *Earth-Science Reviews*, vol. 123, pp. 1–17, 2013. DOI: 10.1016/j.earscirev.2013.04.003.

[20] R. T. Armstrong, H. Ott, A. Georgiadis, M. Rücker, A. Schwing, and S. Berg, "Subsecond pore-scale displacement processes and relaxation dynamics in multiphase flow," *Water Resources Research*, vol. 50, no. 12, pp. 9162–9176, 2014. DOI: 10.1002/2014WR015858.

[21] Y. Gao, Q. Lin, B. Bijeljic, and M. J. Blunt, "X-ray Microtomography of Intermittency in Multiphase Flow at Steady State Using a Differential Imaging Method," *Water Resources Research*, vol. 53, no. 12, pp. 10 274–10 292, 2017. DOI: 10.1002/2017WR021736.

[22] C. Harris, S. J. Jackson, G. P. Benham, S. Krevor, and A. H. Muggeridge, "The impact of heterogeneity on the capillary trapping of $CO_2$ in the Captain Sandstone," *International Journal of Greenhouse Gas Control*, vol. 112, p. 103 511, 2021. DOI: 10.1016/j.ijggc.2021.103511.

[23] M. Dale, S. Ekrann, J. Mykkeltveit, and G. Virnovsky, "Effective Relative Permeabilities and Capillary Pressure for One-Dimensional Heterogeneous Media," *Transport in Porous Media*, vol. 26, no. 3, pp. 229–260, 1997. DOI: 10.1023/A:1006536021302.
